# Supplementary material for: 0ptical trapping with optical magnetic field and photonic Hall effect forces
Source: arXiv:2408.09707 source file (2024-08-19)

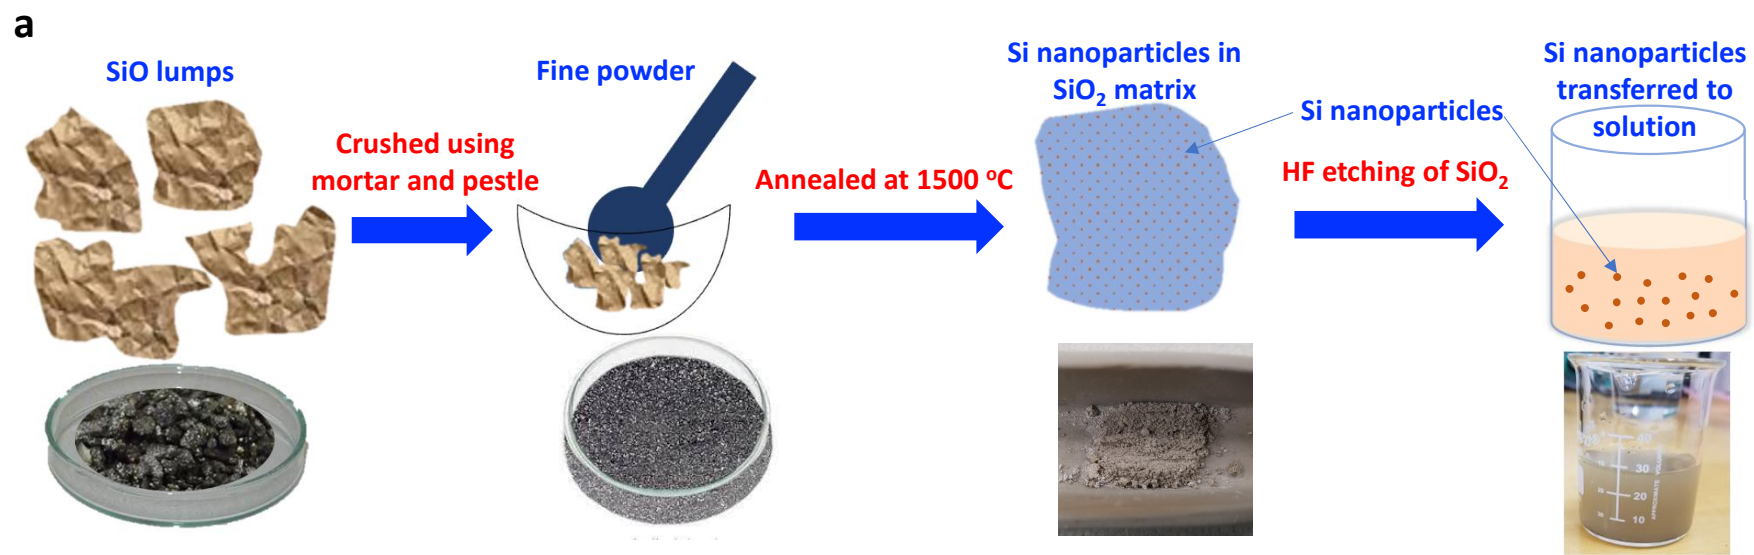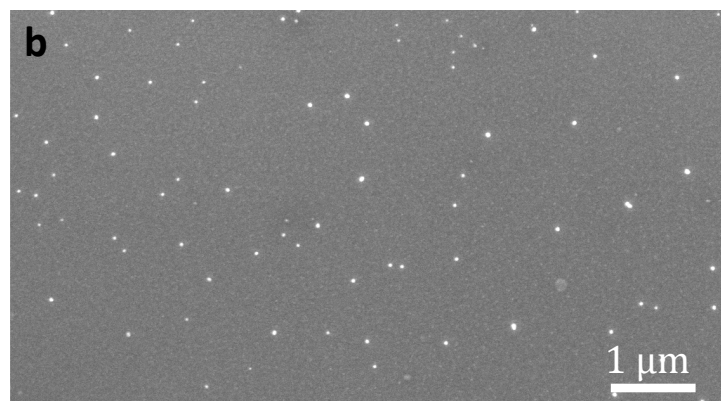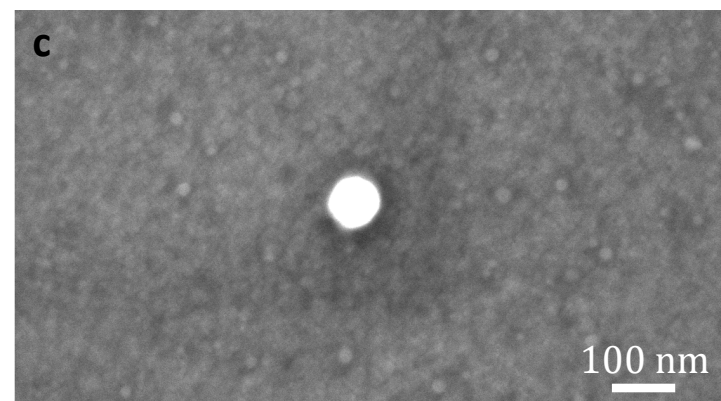

Size Distribution by Intensity

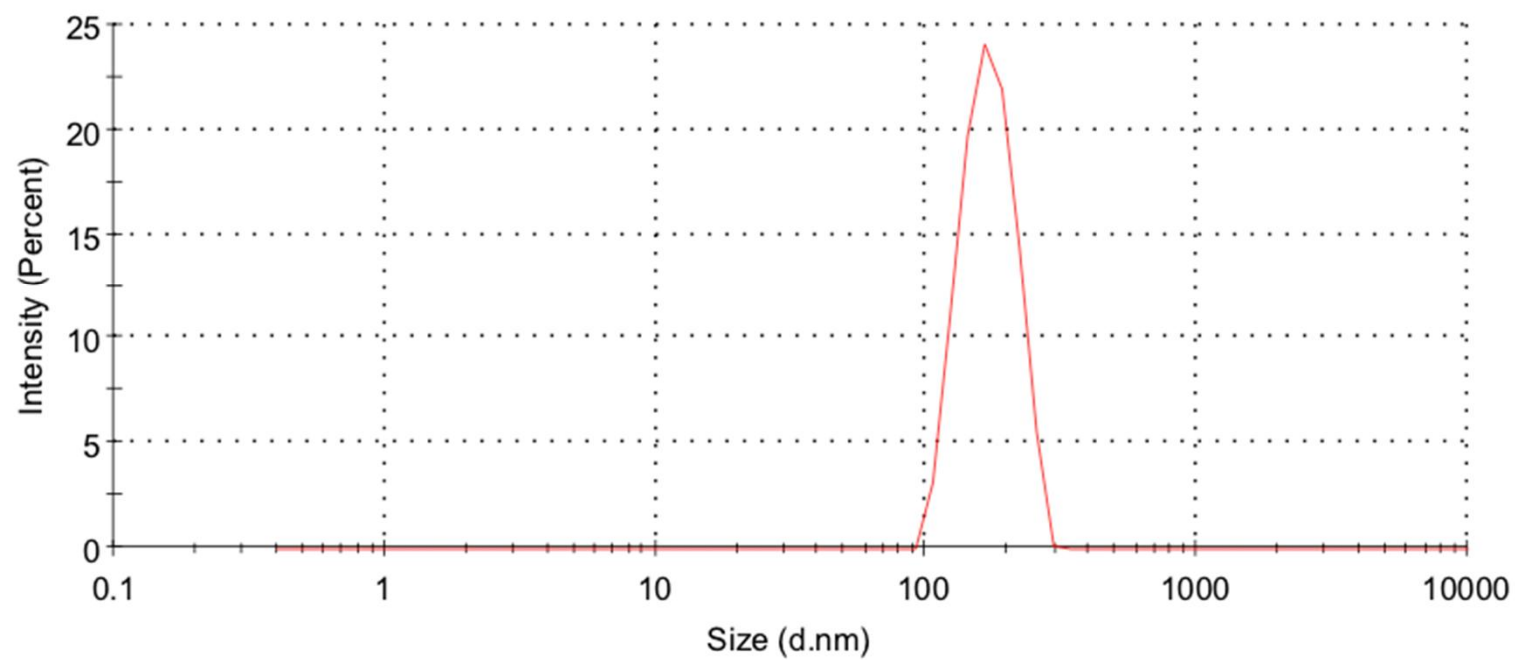

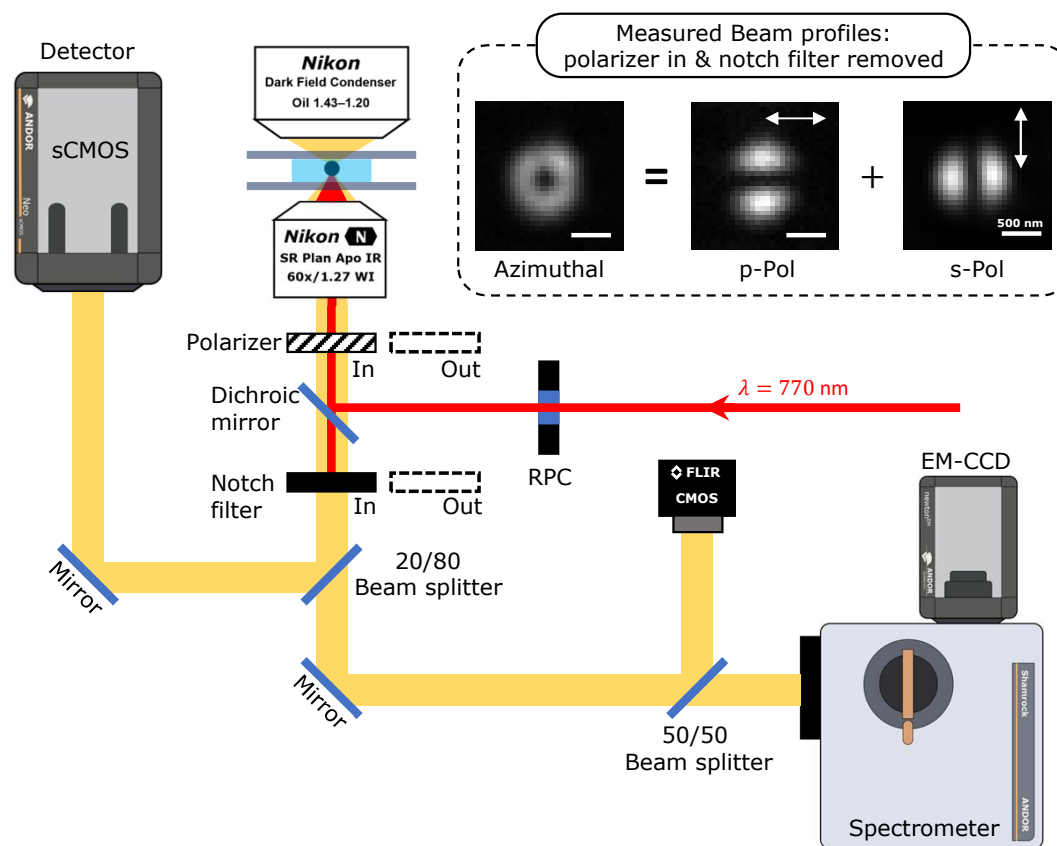

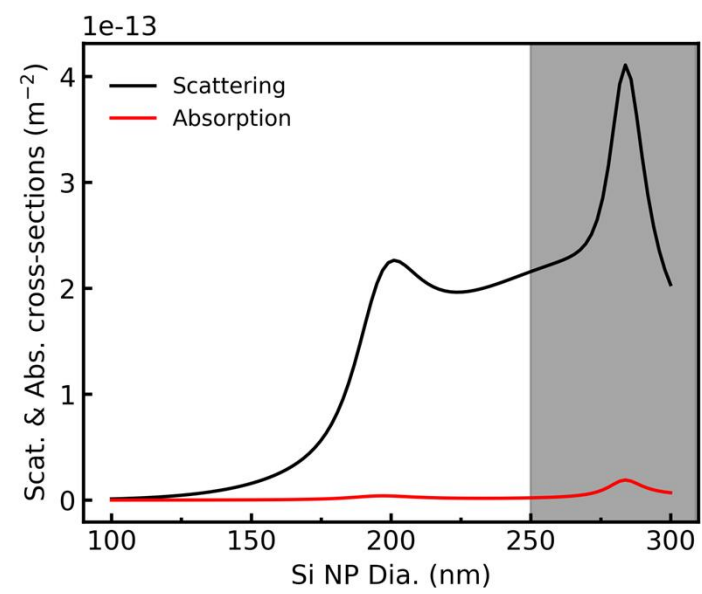

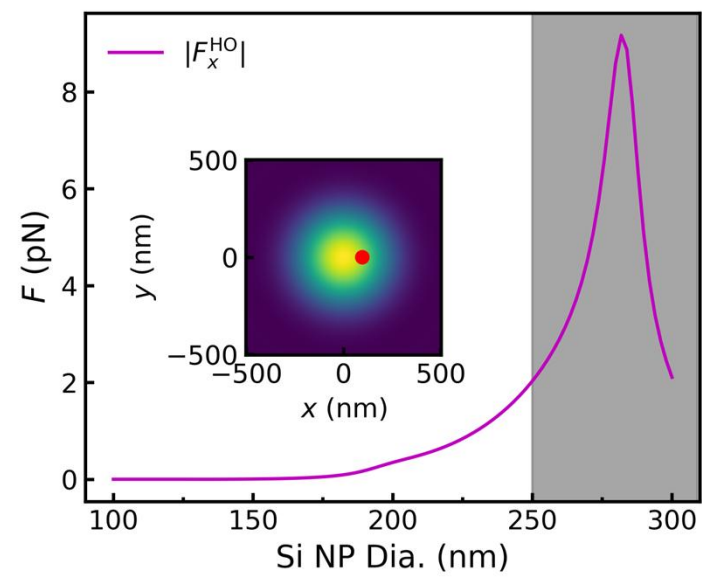

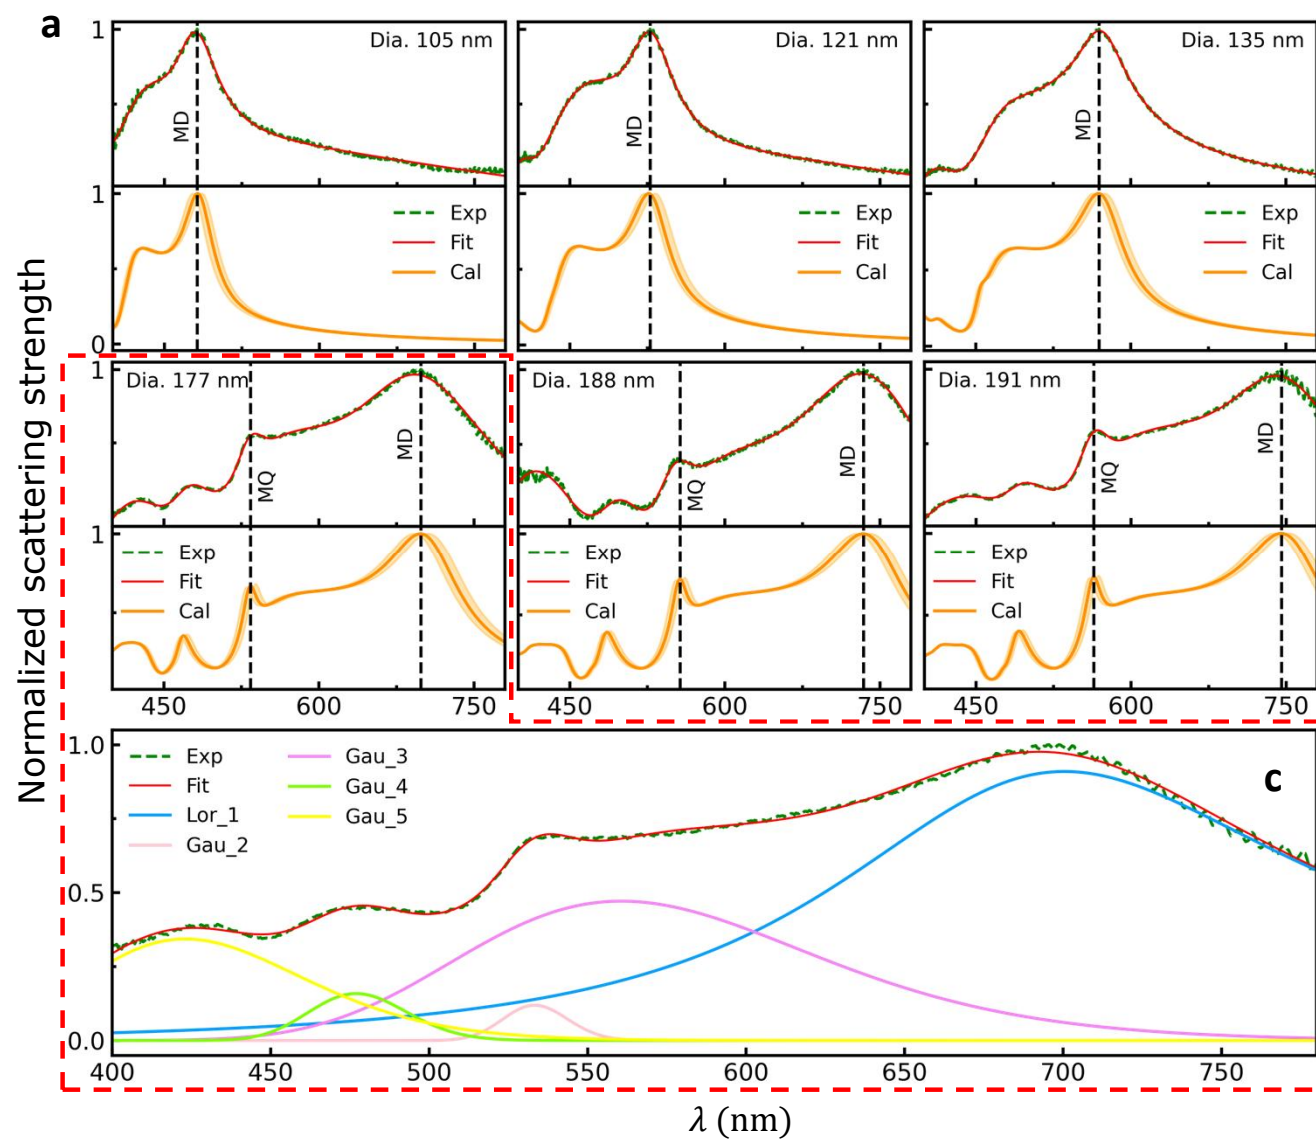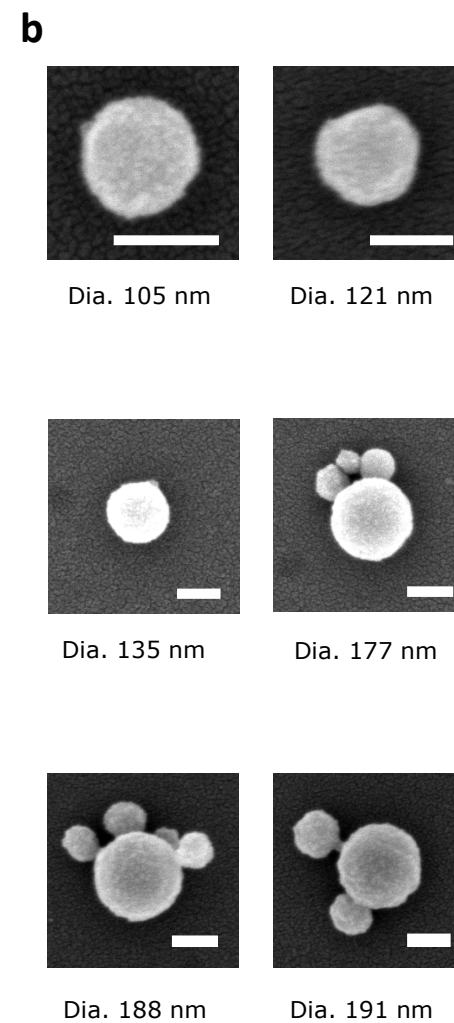

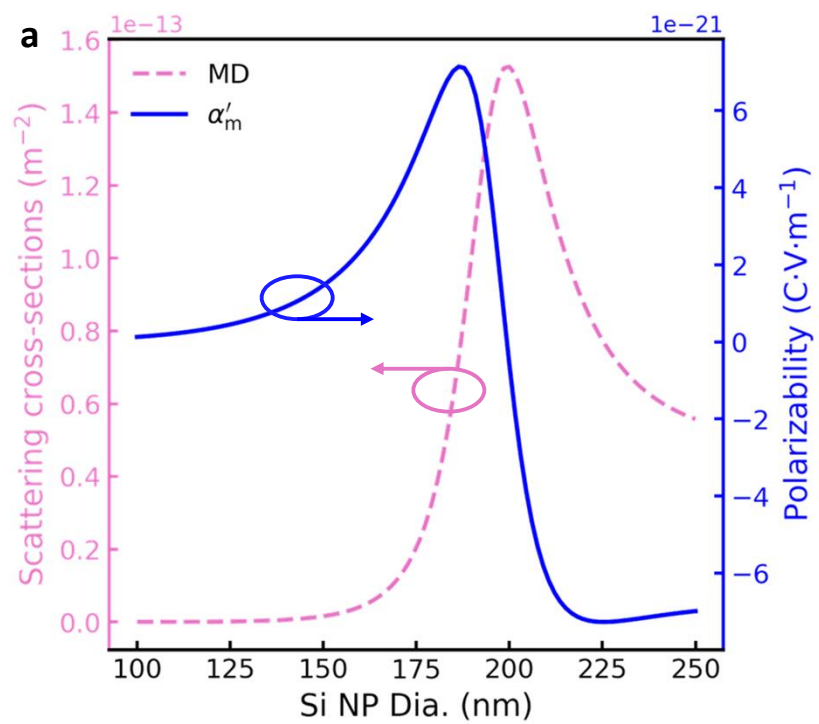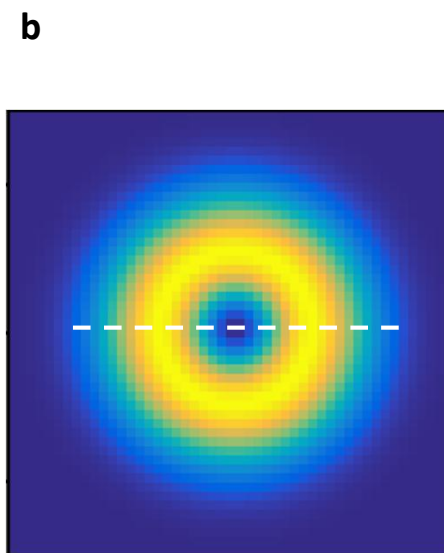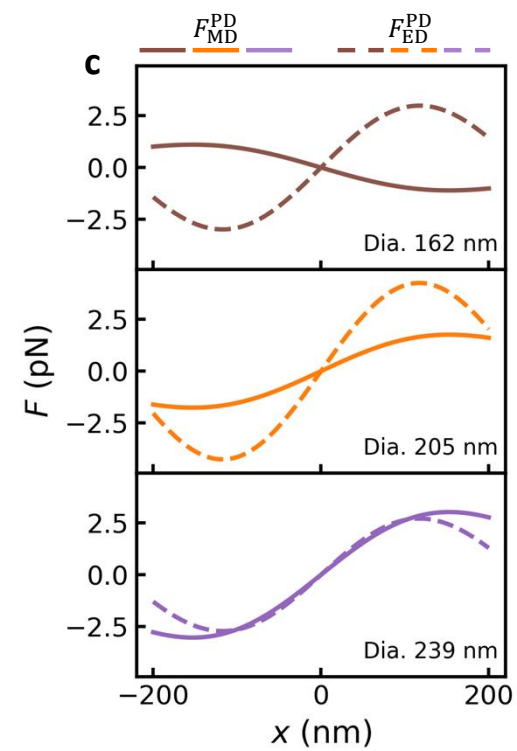

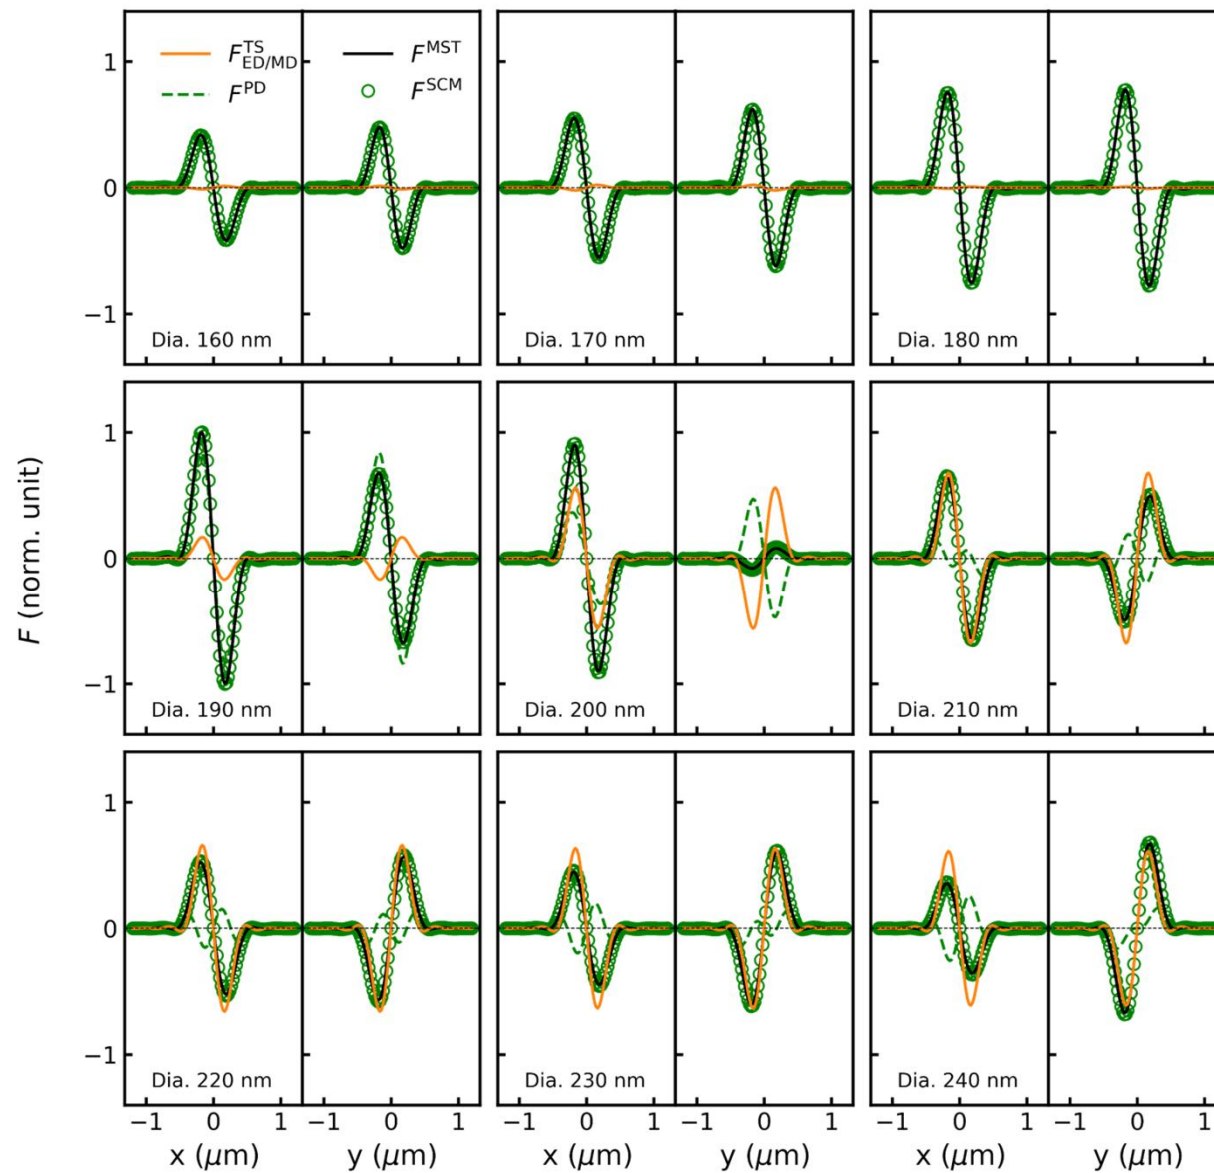



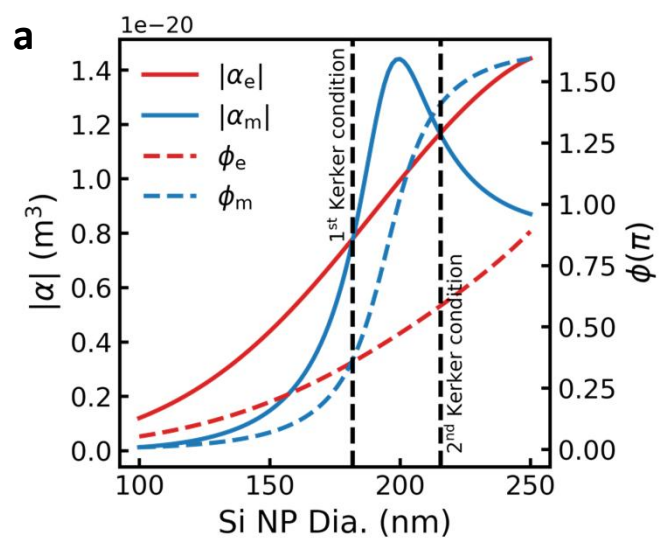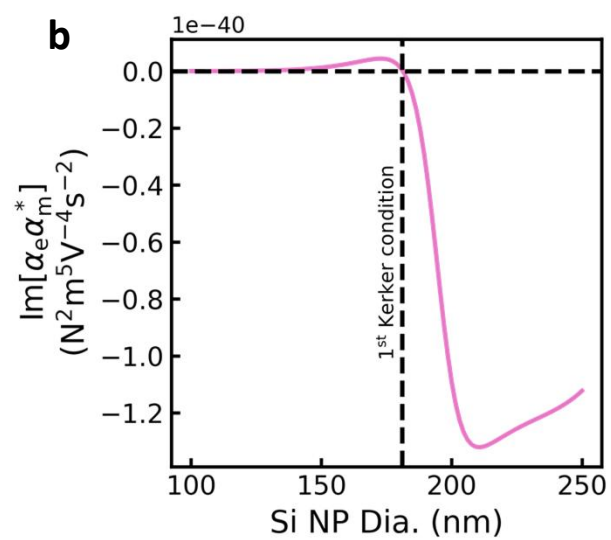

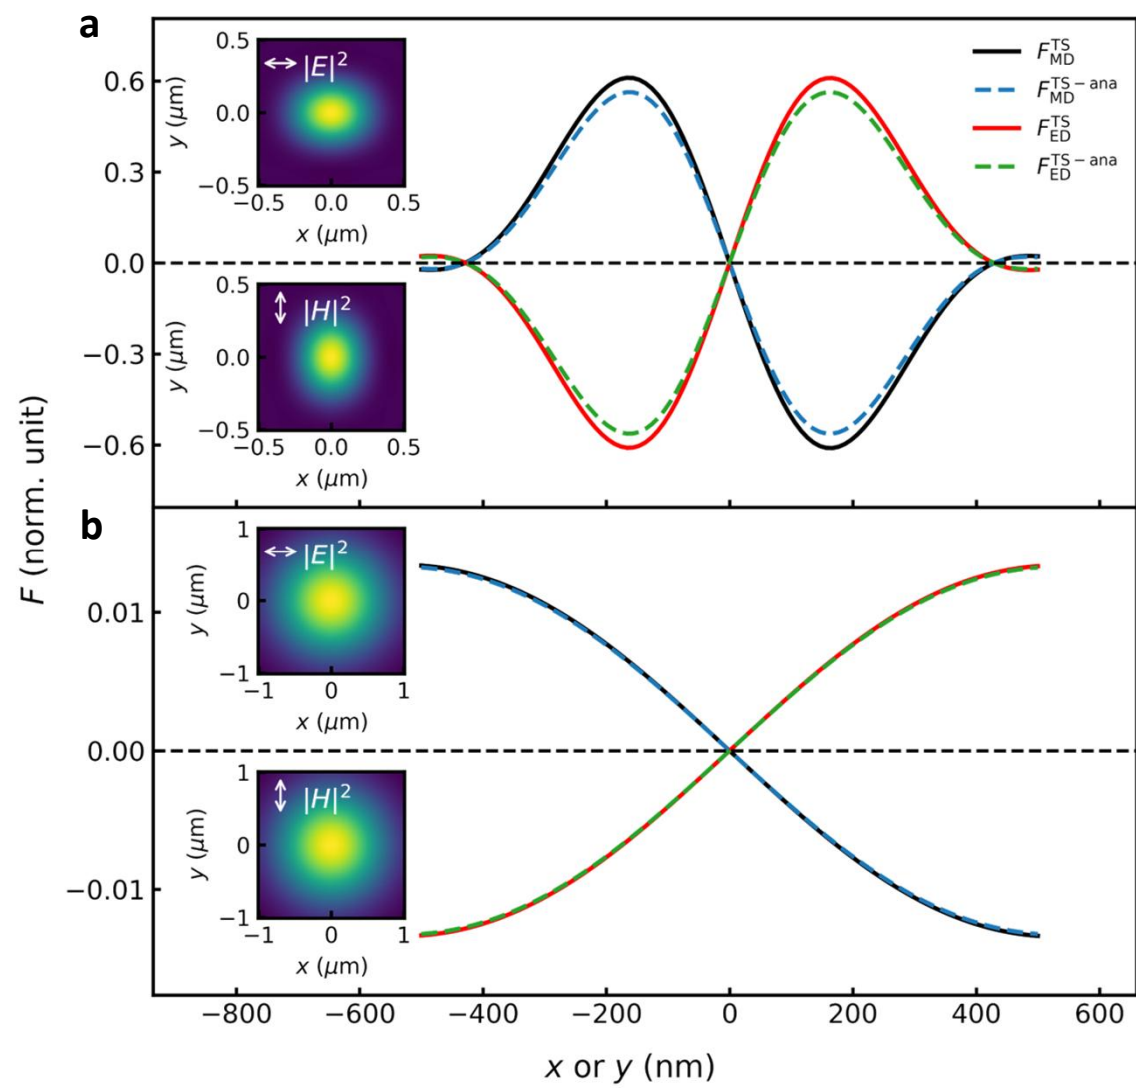

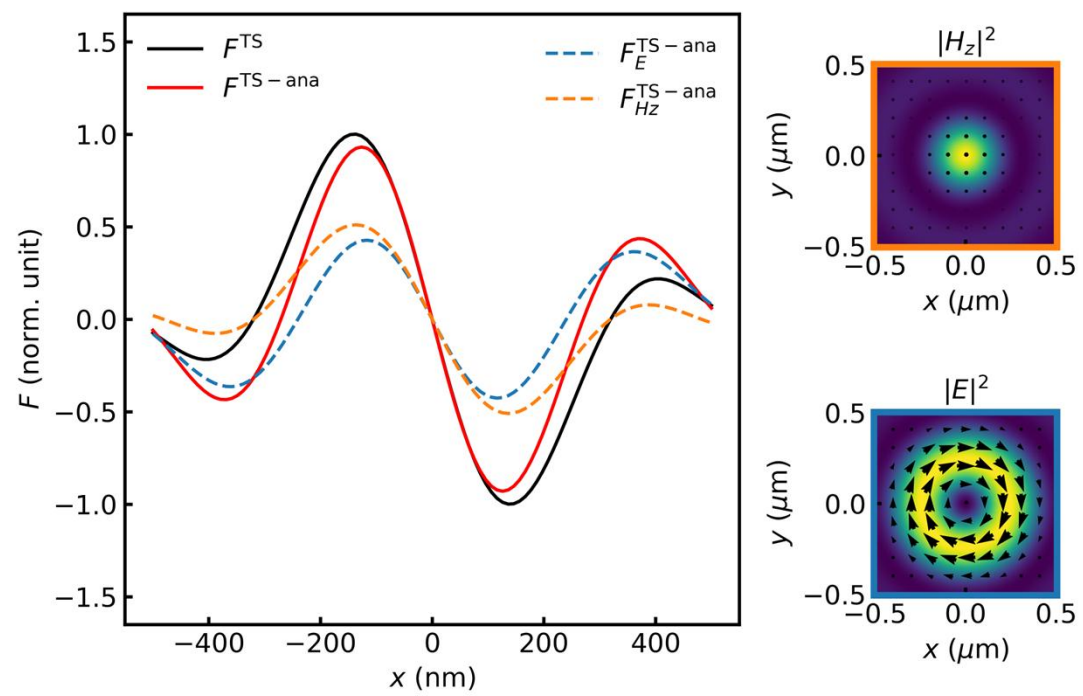

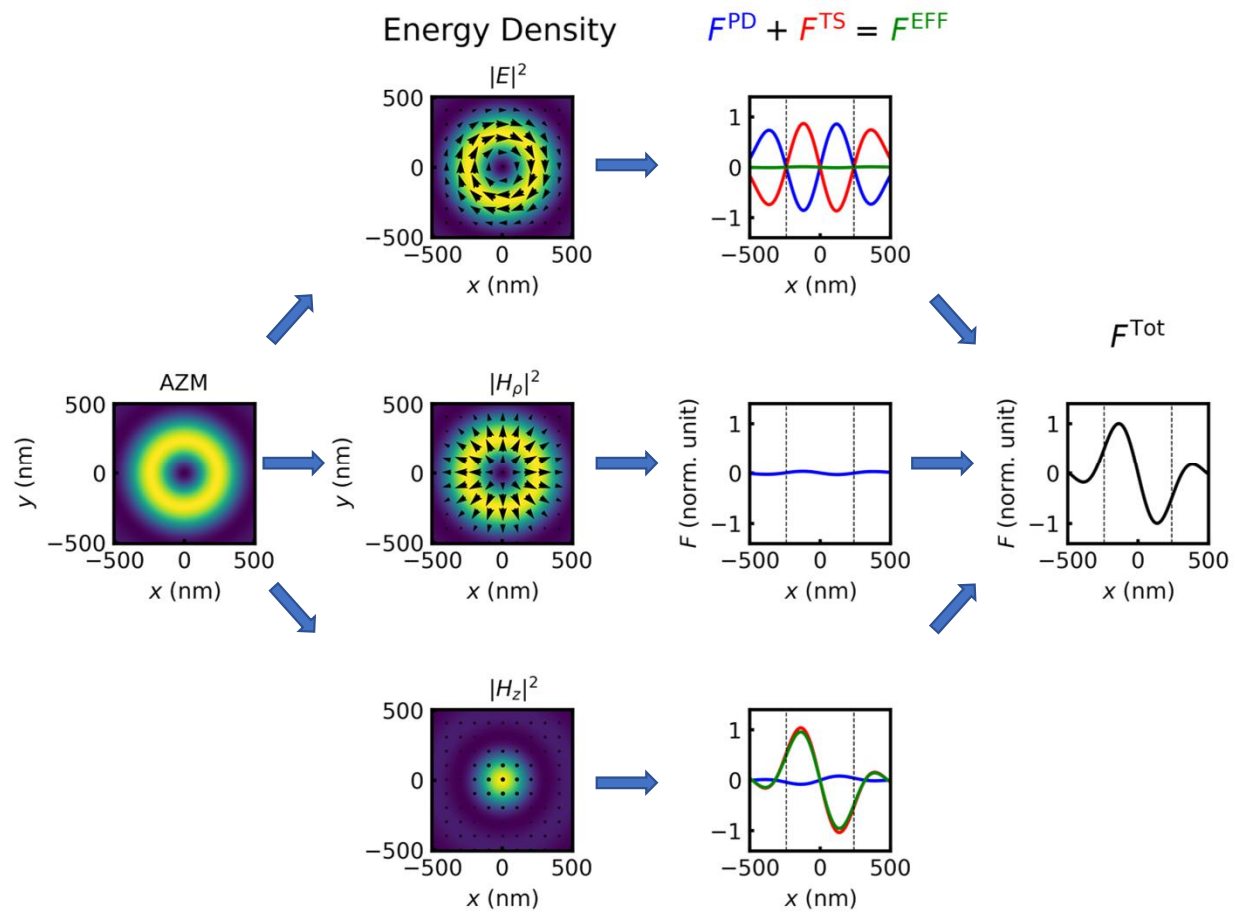

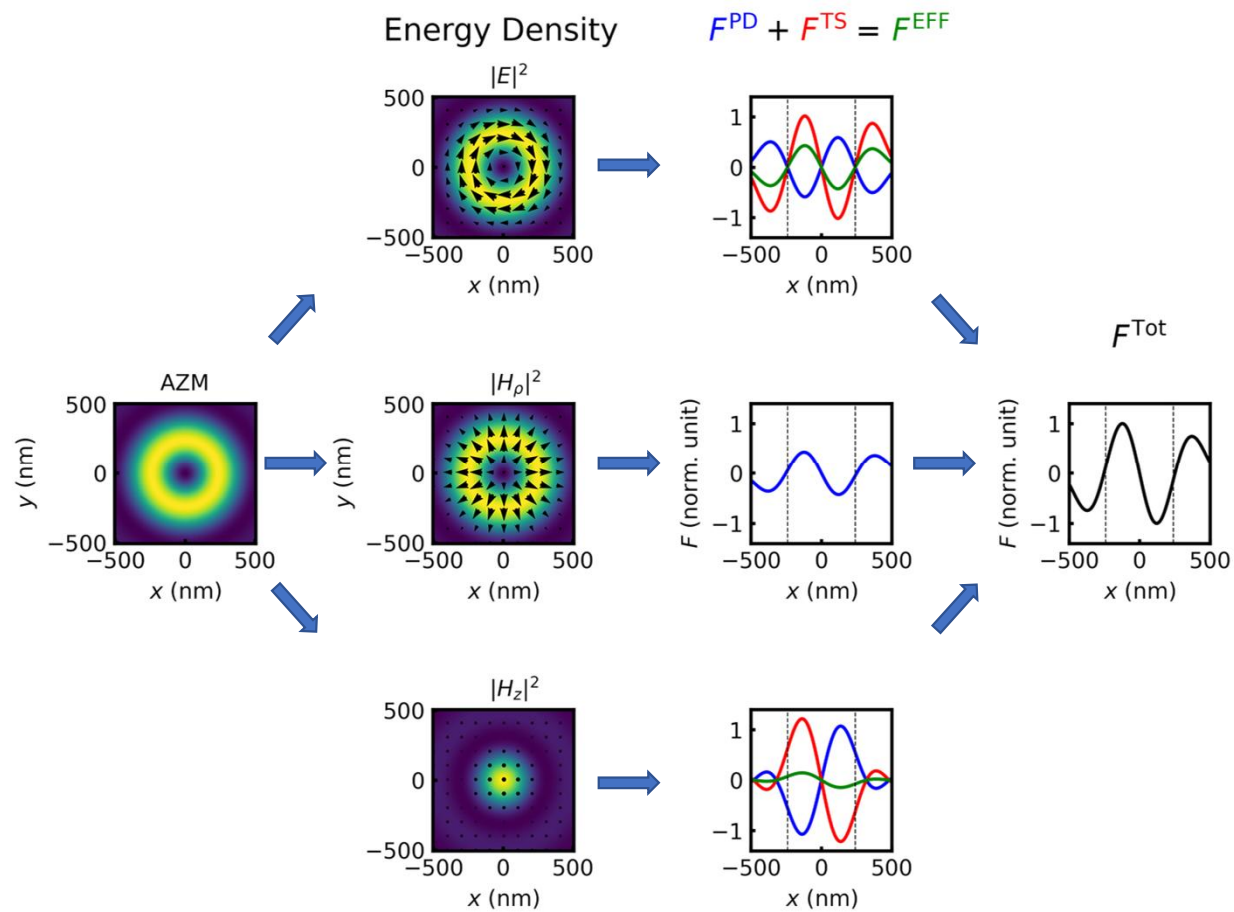

Supplement: Supplementary file 1 [file fig_SI.pdf]
